# Supplementary material for: Local density approximation for excited states
Source: arXiv:2306.04023 source file (2024-06-10)
Supplement: Supplementary file 1 [file HEG-SuppMat.pdf]

# Supplementary material for "Local density approximation for excited states"

Tim Gould
*Queensland Micro- and Nanotechnology Centre, Griffith University, Nathan, Qld 4111, Australia**

Stefano Pittalis
*CNR-Istituto Nanoscienze, Via Campi 213A, I-41125 Modena, Italy*

I) Additional theory about effective occupation factors; II) Additional theory and technical details about the calculations; III) Additional theoretical analysis of similarities in TDLDA and eLDA.

## I. EFFECTIVE OCCUPATION FACTOR

As shown in the main text, the 'trivial' occupation factor model, $\bar{f} \equiv [\sum_i f_i^2 n_i]/[\sum_i f_i n_i] \equiv n^{(2)}/n$, [here and henceforth, $n^{(p)} := \sum_i f_i^p n_i$] gives rather different results to LSDA in doublet ground states. In fact, this expression also has another less obvious problem – it has the wrong dependence in densities. To understand this point, consider the fact that the spin-enhancement for weakly-polarized ($\zeta \to 0^+$) gases varies as $1 + \frac{2}{9}\zeta^2$, while the cofe-enhancement in the same regime ($\bar{f} \to 2^-$) varies as $1 + \frac{2-\bar{f}}{6}$. Since $\zeta = \frac{n_\uparrow - n_\downarrow}{n}$ we see that, $2 - \bar{f}$ should vary as a 'square' of density ratios to match the series expansion in $\zeta$.

Once we recognise that $\bar{f}$ should depend on a ratio 'squared', we may also notice that any model of form,

$$\bar{f}[\{n_i\}; a, b] \equiv \left(\frac{\sum_i f_i^a n_i}{\sum_i f_i n_i}\right)\left(\frac{\sum_i f_i^b n_i}{\sum_i f_i n_i}\right) \equiv \frac{n^{(a)} n^{(b)}}{n^2} \tag{1}$$

will correctly reproduce the HEG $\bar{f}$ provided $a + b = 3$. The HEG result follows from the fact that planewaves have constant densities so yield $\bar{f}[a, b] = \bar{f}^a \bar{f}^b / \bar{f}^2 = \bar{f}^{a+b-2}$.

To determine $a$ (and thus $b$), we use the case of a single unpaired electron as a 'norm', i.e. an approximate constraint used to guide the model toward good properties. Any two-electron has a density, $n = 2n_{\text{Core}} + n_{\text{Frontier}}$, where $n_{\text{Core}} = \sum_{i=0}^{\text{Frontier}-1} n_i$ is the spin-resolved density of paired electrons and $n_{\text{Frontier}}$ is the density of the unpaired frontier electron. Given the ratio, $r = n_{\text{Frontier}}/n_{\text{Core}}$, of frontier to core densities, we may straightforwardly show that the spin-polarizability is $\zeta(r) = \frac{r}{2+r}$. We similarly may write, $\bar{f}(r) = \frac{(2^a+r)(2^{3-a}+r)}{(2+r)(2+r)}$, for the effective occupation factor.

We pick $a$ by ensuring that the exchange spin-enhancement,

$$\frac{\epsilon_{\text{x}}^{\text{pol}}(r)}{\epsilon_{\text{x}}^{\text{unpol}}} = \frac{|1 + \frac{r}{2+r}|^{4/3} + |1 - \frac{r}{2+r}|^{4/3}}{2} \approx \frac{\epsilon_{\text{x}}^{\text{cofe}}(r)}{\epsilon_{\text{x}}^{\text{unpol}}} = \left[\frac{2(2+r)(2+r)}{(2^a + r)(2^{3-a} + r)}\right]^{1/3} \tag{2}$$

of doublets is approximately the same in LSDA and eLDA for all ratios, $0 < r < \infty$. Remarkably, $a = \frac{1}{3}$ (and thus $b = \frac{8}{3}$) is an excellent approximation, giving errors of under 1% for all $r$. Thus, we employ,

$$\bar{f}[\{n_i\}](\boldsymbol{r}) := \left(\frac{\sum_i f_i^{1/3} n_i(\boldsymbol{r})}{\sum_i f_i n_i(\boldsymbol{r})}\right)\left(\frac{\sum_i f_i^{8/3} n_i(\boldsymbol{r})}{\sum_i f_i n_i(\boldsymbol{r})}\right) \equiv \frac{n^{(1/3)}(\boldsymbol{r}) n^{(8/3)}(\boldsymbol{r})}{n(\boldsymbol{r})^2} , \tag{3}$$

as the effective occupation factor for inhomgeneous systems.

## II. MOLECULAR CALCULATIONS

### Theory

The eLDA [Eq. (43) of the main text] involves exact expressions for ensemble $T_s^{\boldsymbol{w}}$ and $E_{\text{H}}^{\boldsymbol{w}}$ and a cofe-derived local density approximation for $E_{\text{xc}}^{\boldsymbol{w}}$. The ensemble energy can be converted to expressions for a given excited state, $|\kappa\rangle$,

* t.gould@griffith.edu.au

by setting $T_{s,\kappa} := \partial_{w_\kappa} T_s^{\boldsymbol{w}} = T_s[n_\kappa]$ and $E_{\text{H},\kappa} := \partial_{w_\kappa} E_{\text{H}}^{\boldsymbol{w}} = U[n_\kappa] + \Delta E_{\text{H},\kappa}$. [1] $\Delta E_{\text{H}}$ will be discussed in the next paragraph. In all cases, we may adapt Eq. (43) to yield the energy of a selected state, $|\Psi_\kappa\rangle$ using,

$$E_\kappa^{\text{eLDA}} := T_s[n_\kappa] + \int n_\kappa(\boldsymbol{r})v(\boldsymbol{r})d\boldsymbol{r} + U[n_\kappa] + \int n_\kappa(\boldsymbol{r})\epsilon_{\text{xc}}^{\text{cofe}}(r_{s,\kappa}(\boldsymbol{r}), \bar{f}_\kappa(\boldsymbol{r}))d\boldsymbol{r} + \Delta E_{\text{H},\kappa} \; . \tag{4}$$

Here, $n_\kappa$ is the density of the state, $r_{s,\kappa}(\boldsymbol{r})$ is its Wigner-Seitz radius and $\bar{f}_\kappa(\boldsymbol{r})$ is its effective occupation factor defined by Eq. (3). $U[\rho] = \frac{1}{2}\Re\int \rho(\boldsymbol{r})\rho(\boldsymbol{r}')\frac{d\boldsymbol{r}d\boldsymbol{r}'}{|\boldsymbol{r}-\boldsymbol{r}'|}$ is the Coloumb integral from Eq. (2) of the main text.

For singlet, doublet, triplet (etc) ground states, it is readily shown that $\Delta E_{\text{H}} = 0$. In other cases considered in the main text there is an extra Hartree contribution,

$$\Delta E_{\text{H},\kappa} \equiv \sum_{kk'\in\text{act}} F_{kk';\kappa}^{K} \tfrac{1}{2} K_{kk'} \; , \qquad K_{kk'} = \Re\int \phi_k(\boldsymbol{r})\phi_{k'}^*(\boldsymbol{r})\phi_k^*(\boldsymbol{r}')\phi_{k'}(\boldsymbol{r}')\frac{d\boldsymbol{r}d\boldsymbol{r}'}{|\boldsymbol{r}-\boldsymbol{r}'|} \tag{5}$$

that is formed out of (complex-adapted) exchange integrals, $K_{kk'}$, where $F_{kk',\kappa}^K$ are factors that depend on the specific system. For single and double promotions from orbital $i$ to orbital $a$ (i.e. excited states of form, $\frac{1}{\sqrt{2}}[\hat{P}_{i\downarrow}^{a\downarrow} - \hat{P}_{i\uparrow}^{a\uparrow}]|\Psi_0\rangle$ and $\hat{P}_{i\downarrow}^{a\downarrow}\hat{P}_{i\uparrow}^{a\uparrow}|\Psi_0\rangle$, where $\hat{P}$ is an orbital promotion operator) we obtain non-zero $F_{ia}^K = F_{ai}^K = 2$ and thus $\Delta E_{\text{H},\kappa} := 2K_{is}$.

The use of $\bar{f}$ and (where relevant) presence of $\Delta E_{\text{H}}$ in Eq (4) make it an *implicit* functional of the density. This leads to orbital-dependent effective Fock operators, defined via $\hat{F}_i\phi_i \equiv \frac{1}{f_i}\frac{\delta E_\kappa^{\text{cofe}}}{\delta\phi_i^*}$, and of specific form,

$$\hat{F}_{i;\kappa} := \hat{t} + v + v_{\text{H}}[n_\kappa] + \left[\epsilon_{\text{xc}}^{\text{cofe}}(r_{s,\kappa}, \bar{f}_\kappa) - \frac{r_{s,\kappa}}{3}\epsilon_{\text{xc},r_s}^{\text{cofe}}(r_{s,\kappa}, \bar{f}_\kappa) + \frac{n_\kappa}{f_i}\frac{\partial\bar{f}}{\partial n_i}\epsilon_{\text{xc},\bar{f}}^{\text{cofe}}(r_{s,\kappa}, \bar{f}_\kappa)\right] + \sum_k \frac{F_{ik;\kappa}^K}{f_i}\hat{v}_K[n_k] \; , \tag{6}$$

where $\hat{t} \equiv -\frac{1}{2}\nabla^2$ is the one-body kinetic energy operator, $v_{\text{H}}[n] = \int n(\boldsymbol{r}')\frac{d\boldsymbol{r}'}{|\boldsymbol{r}-\boldsymbol{r}'|}$ is an effective Hartree-like potential, $\epsilon_{\text{xc},X} \equiv \partial_X\epsilon_{\text{xc}}$ is a derivative of the eLDA energy density, and $\hat{v}_K[n_j]\phi_i \equiv \Re\int \phi_j^*(\boldsymbol{r}')\phi_i(\boldsymbol{r}')\frac{d\boldsymbol{r}'}{|\boldsymbol{r}-\boldsymbol{r}'|}\phi_j(\boldsymbol{r})$ is an effective exchange-like operator potential. Because $\hat{F}_{i;\kappa}$ is orbital-dependent, standard self-consistent field treatment requires significant adaptation to converge.

For our calculations, we therefore minimize the eLDA for a given state, $\kappa$, by direct orbital optimization, i.e. we seek the set of orbitals, $\{\phi_i\}$ that minimize Eq. (4). This involves seeking orbital solutions, $\{\phi_i\}$, of,

$$\frac{\delta E_\kappa^{\text{eLDA}}[n]}{\delta\phi_i^*(\boldsymbol{r})} := 0, \quad \forall i \; , \qquad \frac{\delta^2 E_\kappa^{\text{eLDA}}[n]}{\delta\phi_i^*(\boldsymbol{r})\delta\phi_j(\boldsymbol{r})} \geq 0, \quad \forall i, j \; . \tag{7}$$

Here, and henceforth we drop explicit mention of $\kappa$ in equations – but note that subsequent steps must be carried out for each target excited state.

To solve these equations, we first express the set of orbitals, $\{\phi_k\}$, by their coefficients, $C_{pk}$, ($\mathbb{C}$ as a matrix) in a *real* basis set labeled by indices $p$. We then iteratively update the orbitals using,

$$\mathbb{C} \to \mathbb{C}\exp(\mathbb{A}) \; , \qquad A_{jk} \equiv \frac{\Delta_{jk}\langle\phi_j|f_j\hat{F}_j - f_k\hat{F}_k|\phi_k\rangle}{\Delta_{jk}^2 + \eta^2} \; , \qquad \Delta_{jk} \equiv 2|f_j - f_k||\langle\phi_j|\hat{F}_j|\phi_j\rangle - \langle\phi_k|\hat{F}_k|\phi_k\rangle| \; , \tag{8}$$

where $\eta$ is a numerical 'renormalization' constant that is set to 0.01 Ha, and $\Delta_{jk}$ is an approximation to the Hessian. [2] The form of $A_{jk} = -A_{kj}$ dictates that it is anti-symmetric and thus orbitals are updated via unitary transformations – extension to complex orbitals involves taking the complex conjugate of $\hat{F}_j$ to obtain an anti-Hermitian matrix $A_{jk} = -A_{kj}^*$. Typically, it takes about 20 cycles to find the minimum to required accuracy.

## Technical details

Unless otherwise noted, LSDA and TDLDA calculations are done using the Vosko, Wilk and Nusair [3] parametrisation of the HEG correlation energy. This is the default choice in almost all quantum chemistry packages so, for atoms and molecules, best represents LSDA "as it is done in practice".

All LSDA calculations and TDLDA calculations for gloyxal, benzoquinone and tetrazine were done using `psi4`. [4, 5] TDLDA calculations for TS12 were done using `pyscf` [6, 7] because testing revealed it handled triplet ground states more reliably than `psi4`. eLDA calculations were done using the PW92-based parametrisation of the main paper,

using a custom code (provided on request) that uses `psi4` to evaluate Fock terms and its grid to compute eLDA terms.

For the ionization potential and TS12 calculations we employed an `aug-cc-pvqz` basis set, due to the presence of free atoms and to ensure consistency with the TS12 reference values for other LDA variants. For the spectral calculations we employed `cc-pvtz` for both eLDA and TDLDA calculations. All calculations are done using density-fitting to accelerate evaluation of Coulomb-like integrals.

## III. IMPLICATIONS OF SIMILAR GAPS IN TDLDA AND ELDA

The numerical examples in the main text provide evidence that the predicted TDLDA and eLDA excitation energies can be very similar for cases of practical interest, especially for the lowest excited state energies. These states necessarily involve the case of a *single* excitation from a singlet ground state (gs) to an excited singlet (sx), as TDLDA cannot deal with double excitations. [8] Thus, each excitation is dominated, in orbital terms, by a state involving promotion of occupied orbital $i$ to virtual orbital $a$. We will proceed to derive the conditions for when TDLDA and eLDA will be similar, and briefly discuss its implications for more sophisticated DFAs.

First let us consider the TDLDA gap. The single-pole approximation [see, e.g., Eq. (5) of Ref. 8] applies to excitations with an highly dominant transition and leads to a predicted excitation energy,

$$\Delta E_{ia}^{\text{TDLDA}} \approx \epsilon_a - \epsilon_i + 2\int \phi_i(\boldsymbol{r})\phi_a^*(\boldsymbol{r})\phi_i^*(\boldsymbol{r}')\phi_a(\boldsymbol{r}')\frac{d\boldsymbol{r}d\boldsymbol{r}'}{|\boldsymbol{r}-\boldsymbol{r}'|} + 2\int n_i(\boldsymbol{r})n_a(\boldsymbol{r})f_{\text{xc,gs}}^{\text{LSDA}}(\boldsymbol{r})d\boldsymbol{r} \tag{9}$$

where $f_{\text{xc,gs}} := \frac{d^2 n\epsilon_{\text{xc}}^{\text{LSDA}}}{dndn}|_{n=n_{\text{gs}}}$. Using $\epsilon_k = \int \phi_k^* \hat{h}\phi_k d\boldsymbol{r} = t_k + \int\{v + v_{\text{H}}[n_{\text{gs}}] + v_{\text{xc,gs}}^{\text{LSDA}}\}n_k d\boldsymbol{r}$ gives,

$$\Delta E_{ia}^{\text{TDLDA}} \approx t_a - t_i + \int\{v(\boldsymbol{r}) + v_{\text{H}}[n_{\text{gs}}](\boldsymbol{r}) + v_{\text{xc,gs}}^{\text{LSDA}}(\boldsymbol{r})\}\{n_a(\boldsymbol{r}) - n_i(\boldsymbol{r})\}d\boldsymbol{r} + 2\int n_i(\boldsymbol{r})n_a(\boldsymbol{r})f_{\text{xc,gs}}^{\text{LSDA}}(\boldsymbol{r})d\boldsymbol{r} + 4K_{ia} \ , \tag{10}$$

where $t_k = \frac{1}{2}\int |\nabla\phi_k|^2 d\boldsymbol{r}$, $n_k = |\phi_k|^2$ and $v_{\text{xc,gs}}^{\text{LSDA}} := \frac{dn\epsilon_{\text{xc}}^{\text{LSDA}}}{dn}|_{n=n_{\text{gs}}}$.

Next, consider the eLDA energy gap. The results of the previous section give,

$$\begin{aligned}\Delta E_{ia}^{\text{eLDA}} =& T_s[n_{\text{sx}}] - T_s[n_{\text{gs}}] + \int v(\boldsymbol{r})\{n_{\text{sx}}(\boldsymbol{r}) - n_{\text{gs}}(\boldsymbol{r})\}d\boldsymbol{r} + U[n_{\text{sx}}] + 4K_{ia} - U[n_{\text{gs}}] \\ &+ \int\{n_{\text{sx}}(\boldsymbol{r})\epsilon_{\text{xc}}^{\text{cofe}}(r_{s,\text{sx}}, \bar{f}_{s,\text{sx}}) - n_{\text{gs}}(\boldsymbol{r})\epsilon_{\text{xc}}^{\text{cofe}}(r_{s,\text{gs}}, \bar{f}_{s,\text{gs}})\}d\boldsymbol{r} \ .\end{aligned} \tag{11}$$

The EDFT equivalent of the single-pole approximation is to assume that the orbitals of the excited state are the same as those of the ground state. Using the definitions of $n_\kappa$, $T_{s,\kappa}$ and $U$ gives,

$$\begin{aligned}\Delta E_{ia}^{\text{eLDA}} \approx& t_a - t_i + \int\{v(\boldsymbol{r}) + v_{\text{H}}[n_{\text{gs}}]\}\{n_a(\boldsymbol{r}) - n_i(\boldsymbol{r})\}d\boldsymbol{r} + U[n_a - n_i] \\ &+ \int\{n_{\text{sx}}(\boldsymbol{r})\epsilon_{\text{xc}}(r_{s,\text{sx}}, \bar{f}_{s,\text{sx}}) - n_{\text{gs}}(\boldsymbol{r})\epsilon_{\text{xc}}(r_{s,\text{gs}}, \bar{f}_{s,\text{gs}})\}d\boldsymbol{r} + 4K_{ia} \ .\end{aligned} \tag{12}$$

where we used the relationships, $n_{\text{sx}} - n_{\text{gs}} = n_a - n_i$ and $U[n_{\text{sx}}] - U[n_{\text{gs}}] = \int v_{\text{H}}[n_{\text{gs}}](n_a - n_i)d\boldsymbol{r} + U[n_a - n_i]$ to eliminate some terms.

Now, we are ready to consider the difference between TDLDA and eLDA predictions. Taking the difference between Eqs (12) and (10) yields,

$$\begin{aligned}\Delta E_{ia}^{\text{eLDA}} - \Delta E_{ia}^{\text{TDLDA}} \approx& U[n_a - n_i] + \int\{n_{\text{sx}}\epsilon_{\text{xc}}^{\text{cofe}}(r_{s,\text{sx}}, \bar{f}_{s,\text{sx}}) - n_{\text{gs}}\epsilon_{\text{xc}}^{\text{cofe}}(r_{s,\text{gs}}, \bar{f}_{s,\text{gs}})\}d\boldsymbol{r} \\ &- \int v_{\text{xc,gs}}^{\text{LSDA}}\{n_a - n_i\}d\boldsymbol{r} - 2\int f_{\text{xc,gs}}^{\text{LSDA}} n_i n_a d\boldsymbol{r} \ ,\end{aligned} \tag{13}$$

as the difference between TDLDA and eLDA gaps. Next, make the Taylor expansion, $n\epsilon_{\text{xc}}^{\text{cofe}}(r_{s,\text{sx}}, \bar{f}_{\text{sx}}) \approx n\epsilon_{\text{xc}}^{\text{cofe}}(r_{s,\text{gs}}, \bar{f}_{\text{sx}}) + (n_a - n_i)v_{\text{xc}}^{\text{cofe}} + \frac{1}{2}(n_a - n_i)^2 f_{\text{xc}}^{\text{cofe}}$, to obtain,

$$\Delta E_{ia}^{\text{eLDA}} - \Delta E_{ia}^{\text{TDLDA}} \approx U[n_a - n_i] + \int\left\{\tfrac{1}{2}(n_a - n_i)^2 f_{\text{xc,gs}}^{\text{cofe}} - 2n_i n_a f_{\text{xc,gs}}^{\text{LSDA}}\right\}d\boldsymbol{r} \ . \tag{14}$$

Here, we made the additional implicit assumption that the xc energy density, $\epsilon_{\text{xc}}$, and potential, $v_{\text{xc}}$ are sufficiently similar (for the relevant transition) in spin-polarized TDLDA and cofe-based eLDA that we can substitute one for the other to leading order. All first order effects therefore cancel out, and the only difference is at second order in the transition densities.

This analysis explains why TDLDA and eLDA often give similar results, even when neither approach makes particularly good predictions. Indeed, TDLDA and eLDA will always yield similar excitation energies when:

1. an excitation is strongly dominated by a single transition from orbital $i$ to $a$;

2. orbitals do not change significantly between the ground and excited states;

3. the second order effect from transition densities is small..

The cases of glyoxal, benzoquinone and tetrazine considered in the main text involve orbitals of different spatial symmetries, and the spatial symmetries help to ensure that conditions 1 and 2 are satisfied. Numerical evidence validates Condition 3.

Importantly, the derivations in this section also apply without change to GGAs and meta-GGAs (MGGAs). Thus, so long as the above conditions above continue to hold when we change DFA, then all changes from the GGA or MGGA are likely to be the same in TDDFT and eDFT. Put another way, whenever TDLDA and eLDA give similar excitation energies, any improvements in the TDGGA or TDMGGA spectra are likely to 'carry across' to the eGGA or eMGGA spectra.


[1] T. Gould, L. Kronik, and S. Pittalis, Double excitations in molecules from ensemble density functionals: Theory and approximations, Phys Rev A **104**, 022803 (2021).

[2] G. Levi, A. V. Ivanov, and H. Jónsson, Variational calculations of excited states via direct optimization of the orbitals in dft, Faraday Discuss. **224**, 448 (2020).

[3] S. H. Vosko, L. Wilk, and M. Nusair, Accurate spin-dependent electron liquid correlation energies for local spin density calculations: a critical analysis, Can J Phys **58**, 1200 (1980).

[4] R. M. Parrish, L. A. Burns, D. G. A. Smith, A. C. Simmonett, A. E. DePrince, E. G. Hohenstein, U. Bozkaya, A. Y. Sokolov, R. D. Remigio, R. M. Richard, J. F. Gonthier, A. M. James, H. R. McAlexander, A. Kumar, M. Saitow, X. Wang, B. P. Pritchard, P. Verma, H. F. Schaefer, K. Patkowski, R. A. King, E. F. Valeev, F. A. Evangelista, J. M. Turney, T. D. Crawford, and C. D. Sherrill, Psi4 1.1: An open-source electronic structure program emphasizing automation, advanced libraries, and interoperability, J. Chem. Theory Comput. **13**, 3185 (2017).

[5] D. G. A. Smith, L. A. Burns, D. A. Sirianni, D. R. Nascimento, A. Kumar, A. M. James, J. B. Schriber, T. Zhang, B. Zhang, A. S. Abbott, E. J. Berquist, M. H. Lechner, L. A. Cunha, A. G. Heide, J. M. Waldrop, T. Y. Takeshita, A. Alenaizan, D. Neuhauser, R. A. King, A. C. Simmonett, J. M. Turney, H. F. Schaefer, F. A. Evangelista, A. E. DePrince, T. D. Crawford, K. Patkowski, and C. D. Sherrill, Psi4numpy: An interactive quantum chemistry programming environment for reference implementations and rapid development, J. Chem. Theory Comput. **14**, 3504 (2018).

[6] Q. Sun, T. C. Berkelbach, N. S. Blunt, G. H. Booth, S. Guo, Z. Li, J. Liu, J. D. McClain, E. R. Sayfutyarova, S. Sharma, S. Wouters, and G. K. Chan, PySCF: the python-based simulations of chemistry framework, WIREs Comput. Mol. Sci. **8**, 10.1002/wcms.1340 (2017).

[7] Q. Sun, X. Zhang, S. Banerjee, P. Bao, M. Barbry, N. S. Blunt, N. A. Bogdanov, G. H. Booth, J. Chen, Z.-H. Cui, J. J. Eriksen, Y. Gao, S. Guo, J. Hermann, M. R. Hermes, K. Koh, P. Koval, S. Lehtola, Z. Li, J. Liu, N. Mardirossian, J. D. McClain, M. Motta, B. Mussard, H. Q. Pham, A. Pulkin, W. Purwanto, P. J. Robinson, E. Ronca, E. R. Sayfutyarova, M. Scheurer, H. F. Schurkus, J. E. T. Smith, C. Sun, S.-N. Sun, S. Upadhyay, L. K. Wagner, X. Wang, A. White, J. D. Whitfield, M. J. Williamson, S. Wouters, J. Yang, J. M. Yu, T. Zhu, T. C. Berkelbach, S. Sharma, A. Y. Sokolov, and G. K.-L. Chan, Recent developments in the PySCF program package, J. Chem. Phys. **153**, 10.1063/5.0006074 (2020).

[8] N. T. Maitra, F. Zhang, R. J. Cave, and K. Burke, Double excitations within time-dependent density functional theory linear response, J. Chem. Phys. **120**, 5932 (2004).
